# Supplementary material for: Measurement of the $B_c^+$ meson lifetime using $B_c^+ \to J\!/\!\psi\mu^+ \nu_{\mu} X$ decays
Source: arXiv:1401.6932 source file (2014-01-27)
Supplement: Supplementary file 1 [file supplementary-app.tex]

\clearpage

\section{Supplementary material}
\label{sec:Supplementary-App}

This appendix includes supplementary material that will be 
  part of the draft during the review phase but will not appear in the
  final version of the paper. Instead it will be posted as supplementary
  material alongside the paper on CDS.

\begin{figure}[!htb]
  \begin{center}
    \includegraphics[width=.9\textwidth]{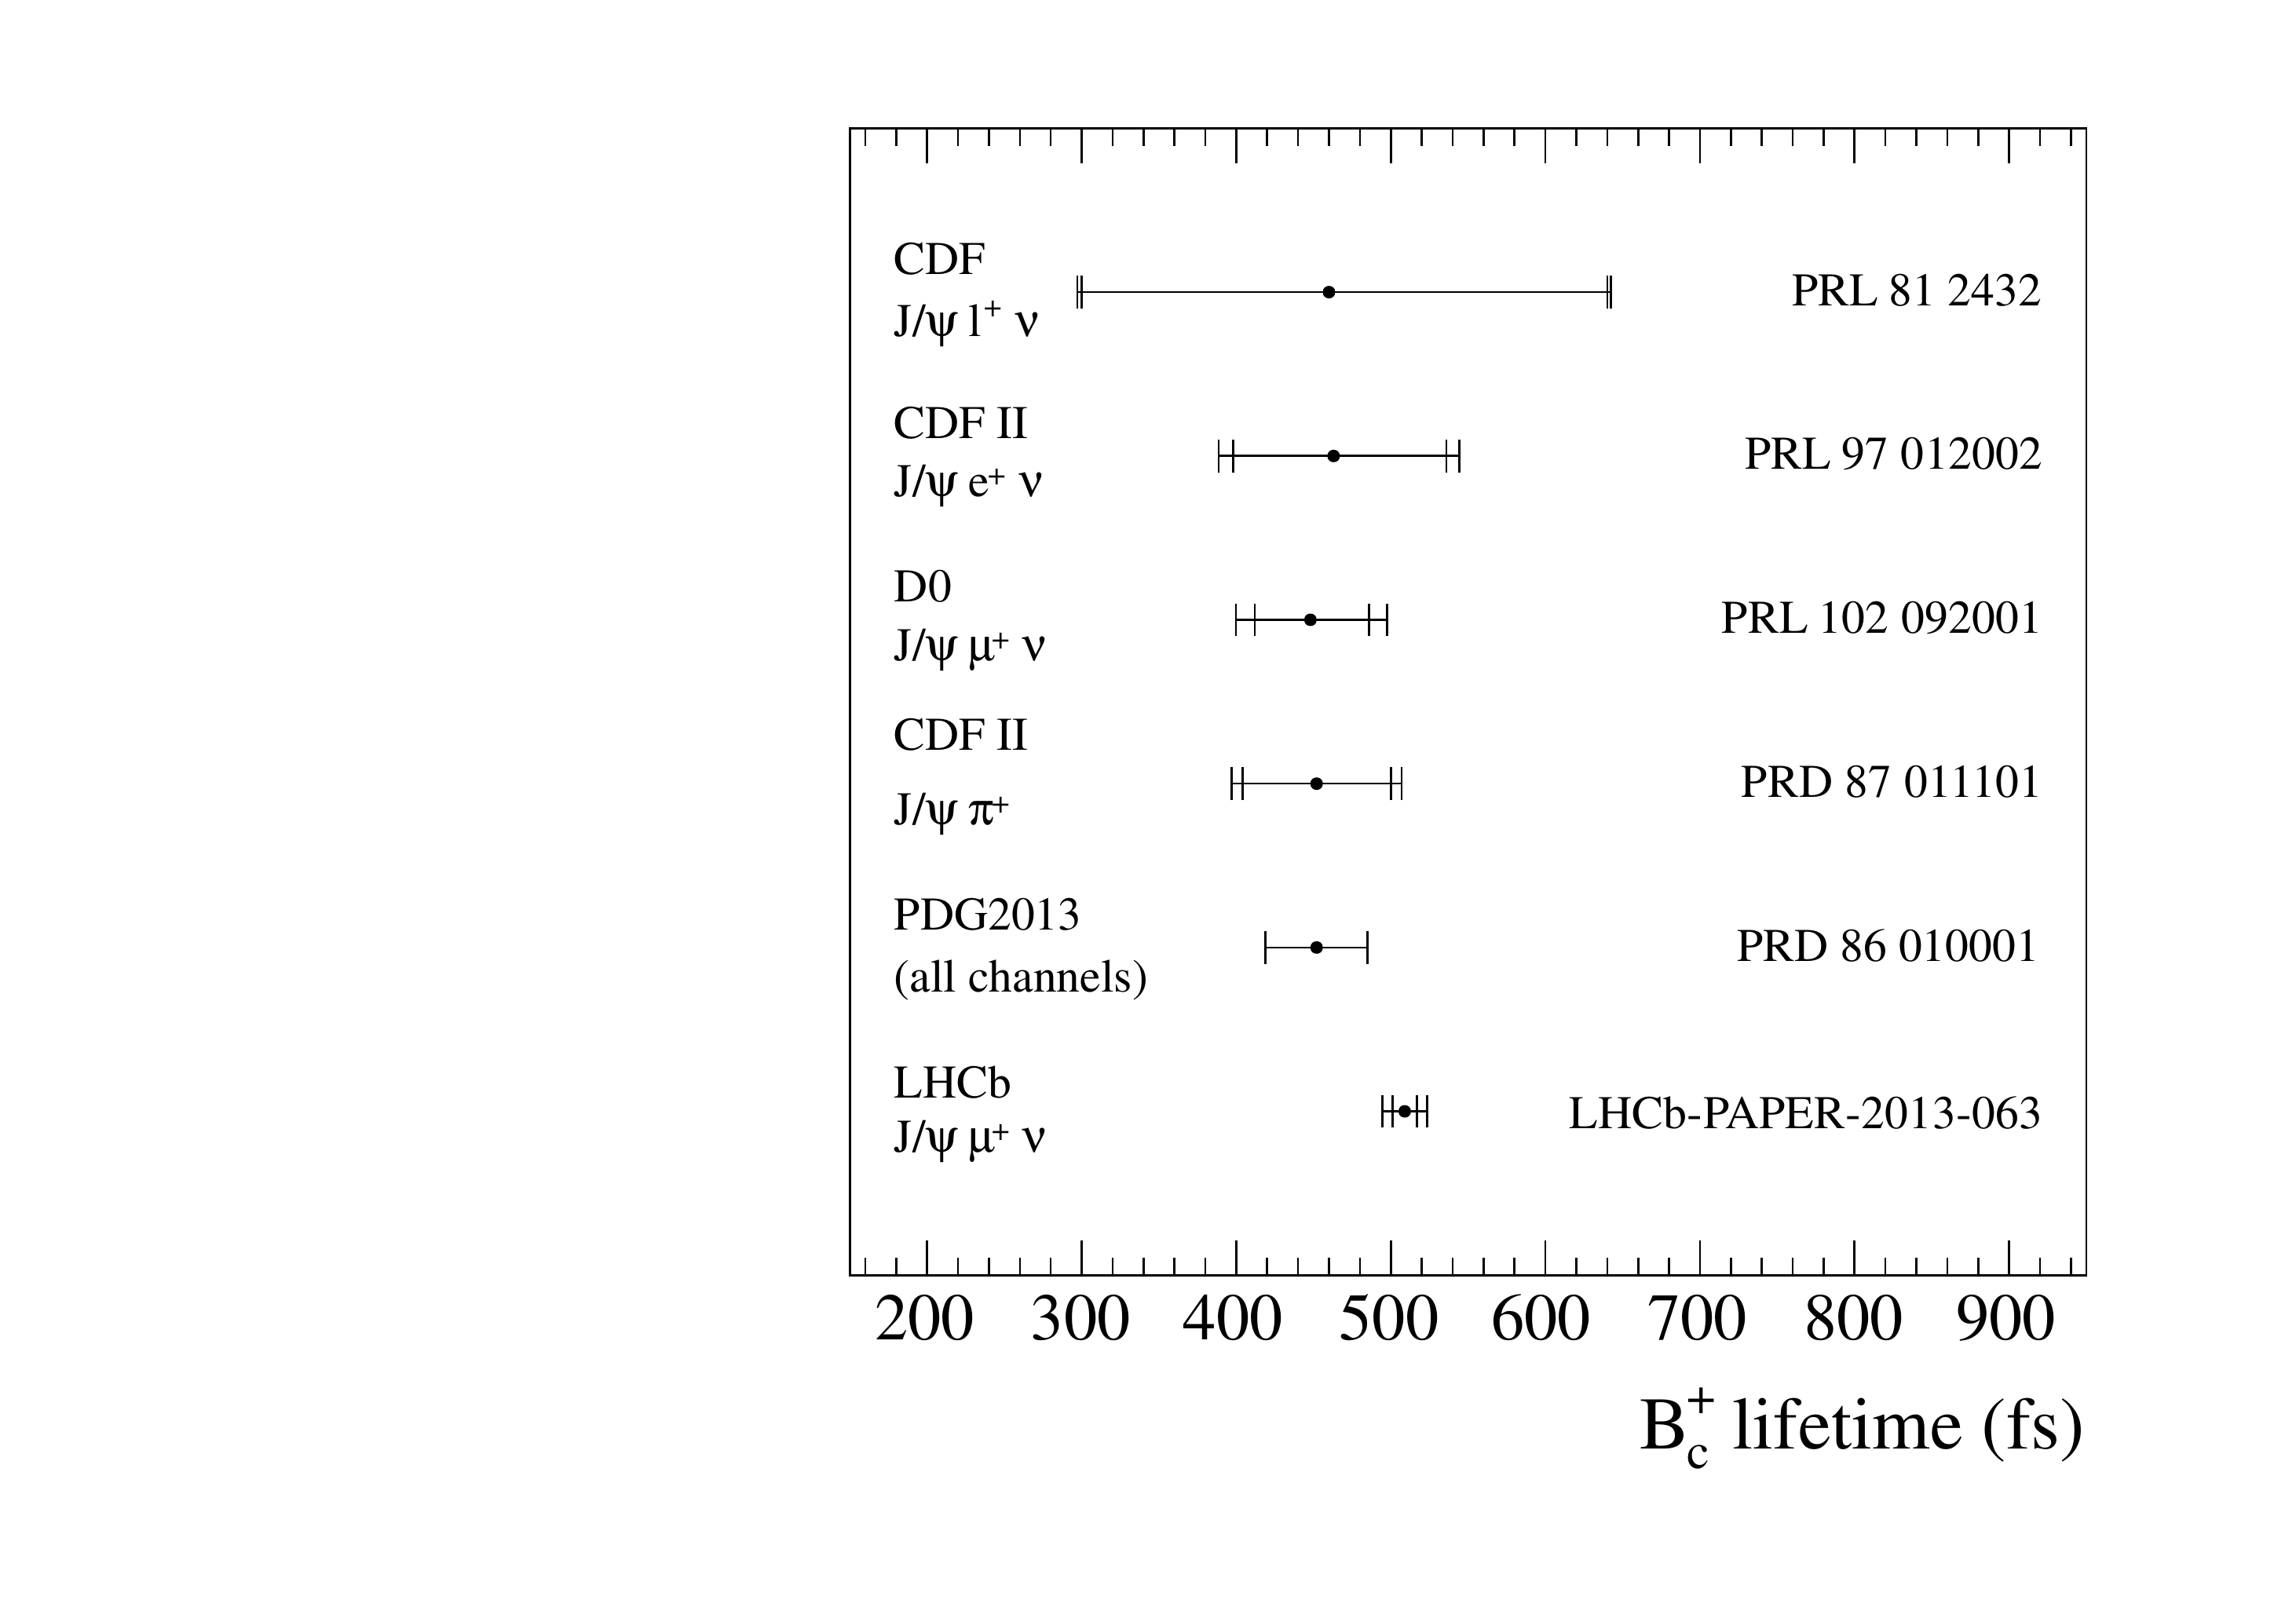}
    \vspace*{-1.0cm}
  \end{center}
  \caption{
    \small     
    Comparison of the result of this determination of the \Bc meson lifetime with those from previous
    measurements~\cite{Abe:1998wi,Abulencia:2006zu,Abazov:2008rba,Aaltonen:2012yb} and with the 2013 PDG average~\cite{PDG2012}.}  
  \label{fig:resultCmp}
\end{figure}

\begin{figure}[p]
  \centering
\includegraphics[width=.73\textwidth]{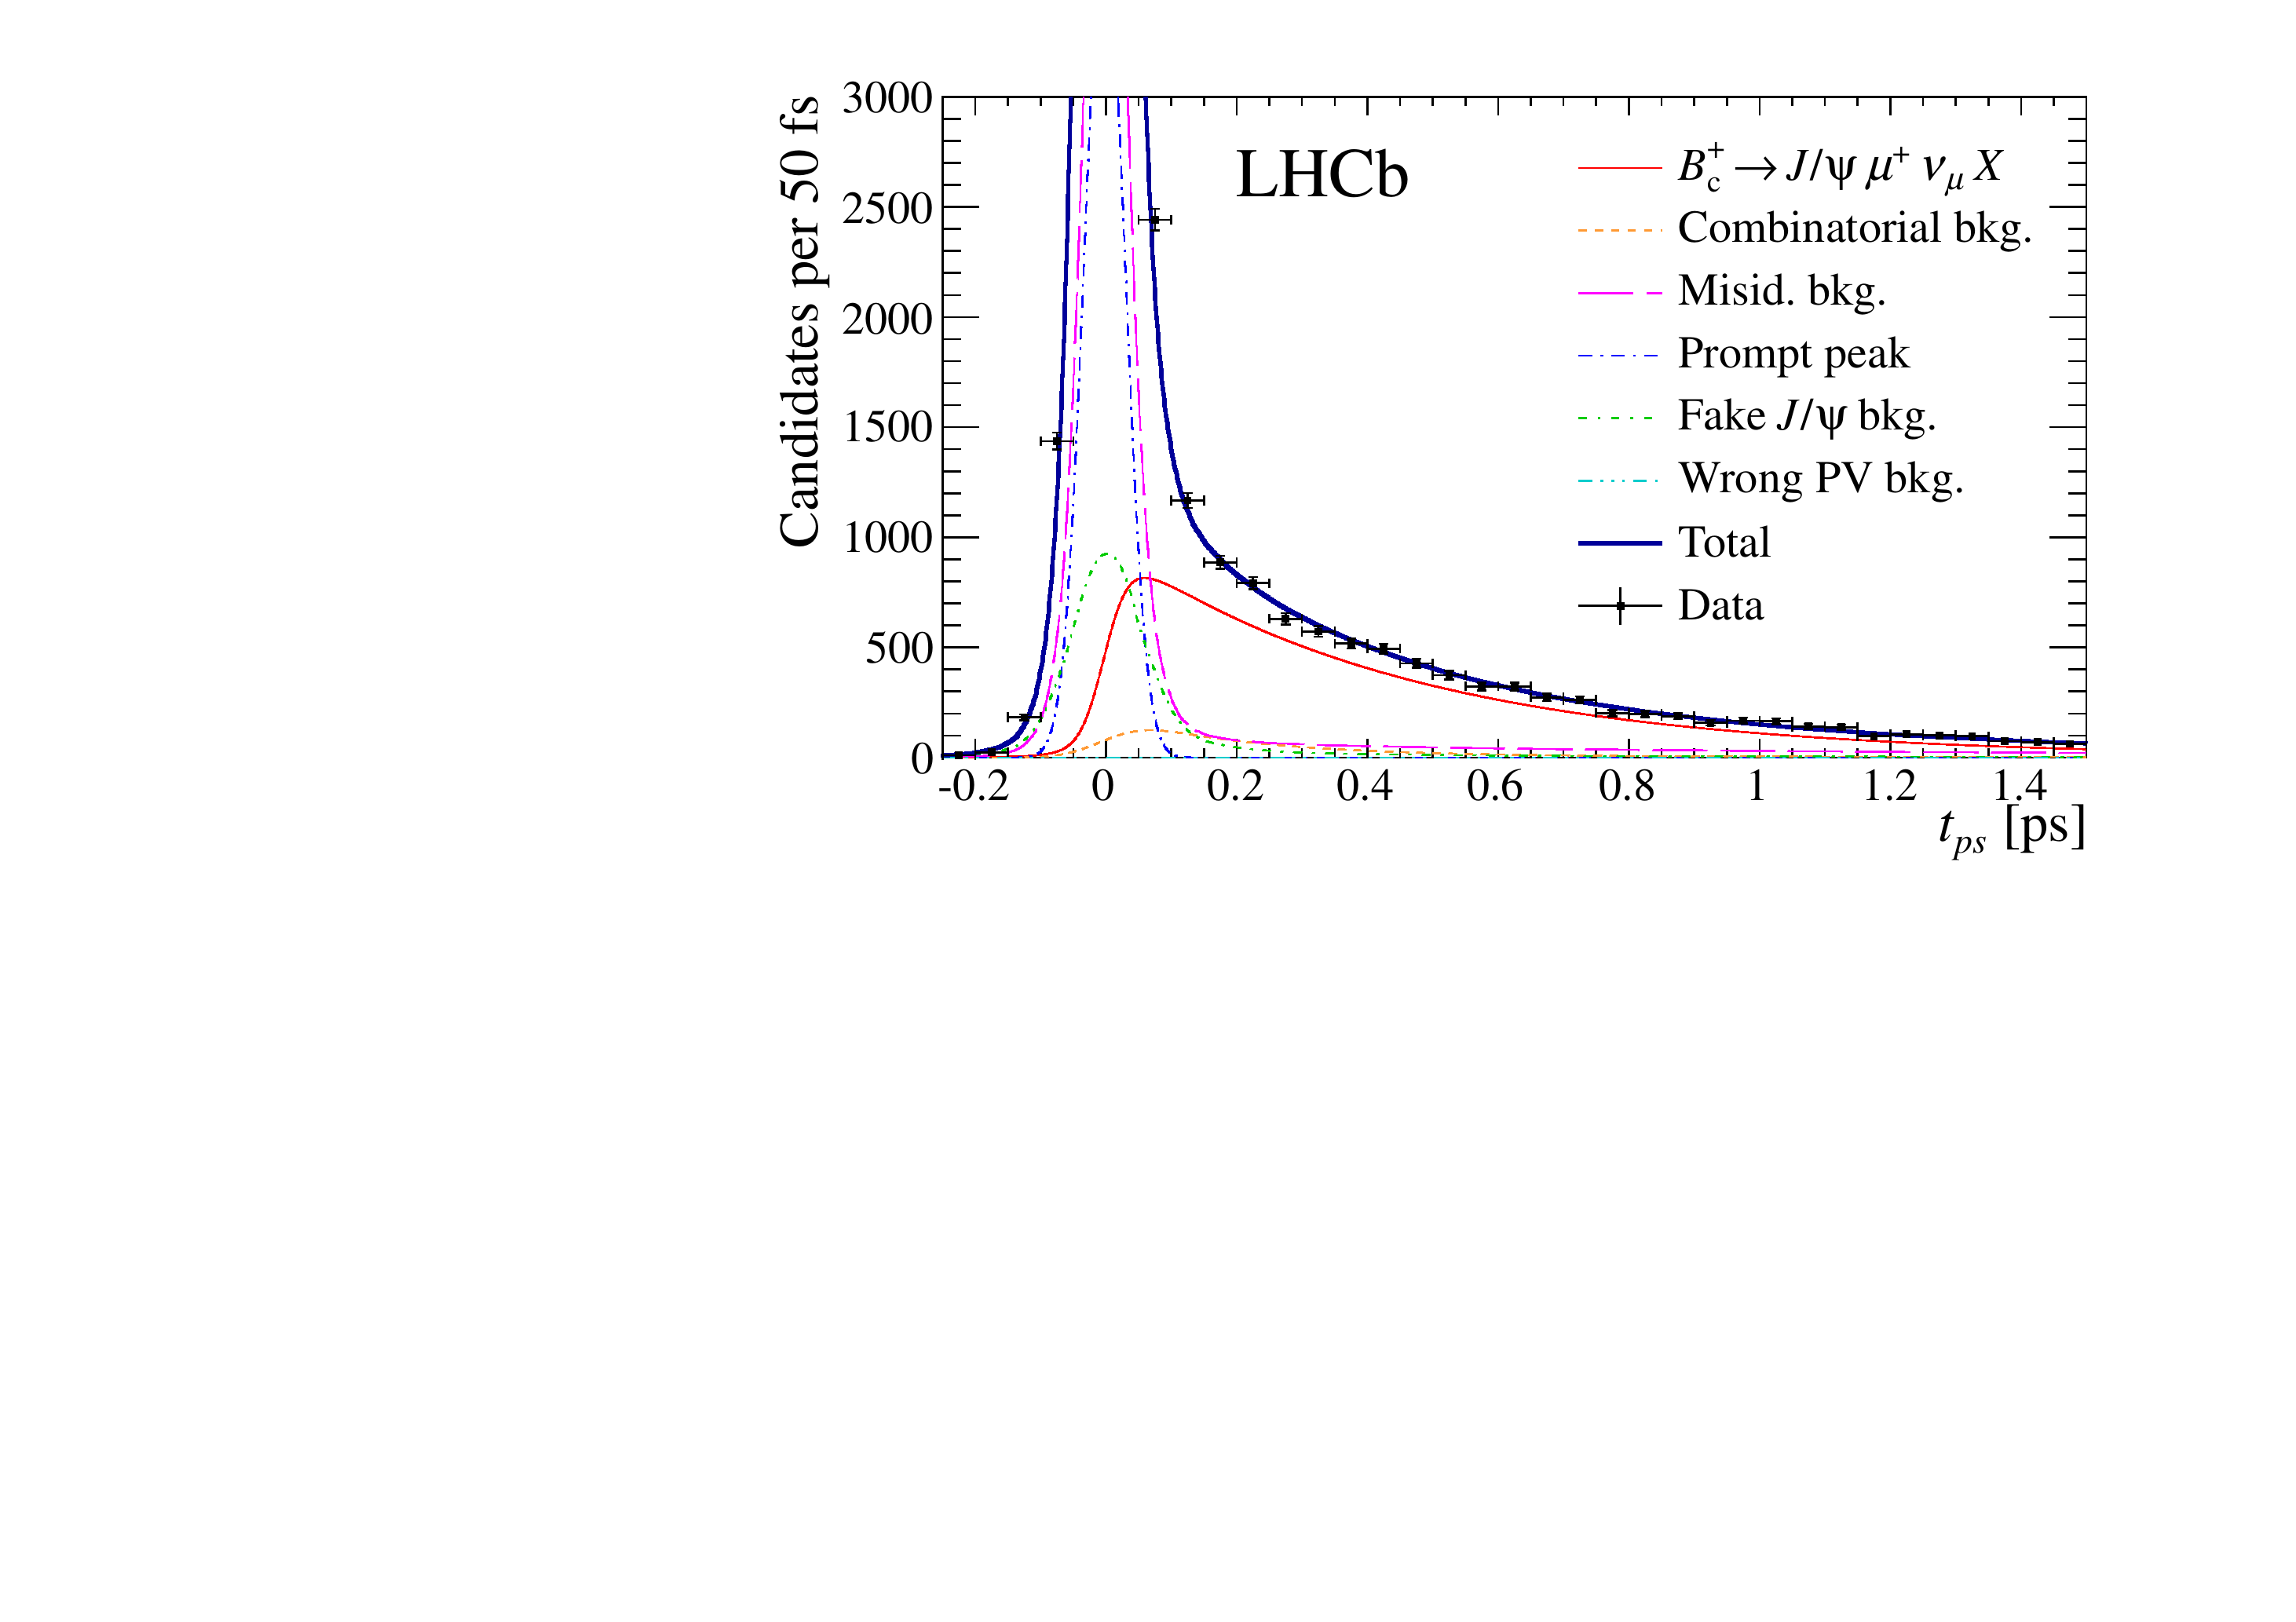}
\put(-200,130){$\mathrm{a})$}\\
\includegraphics[width=.73\textwidth]{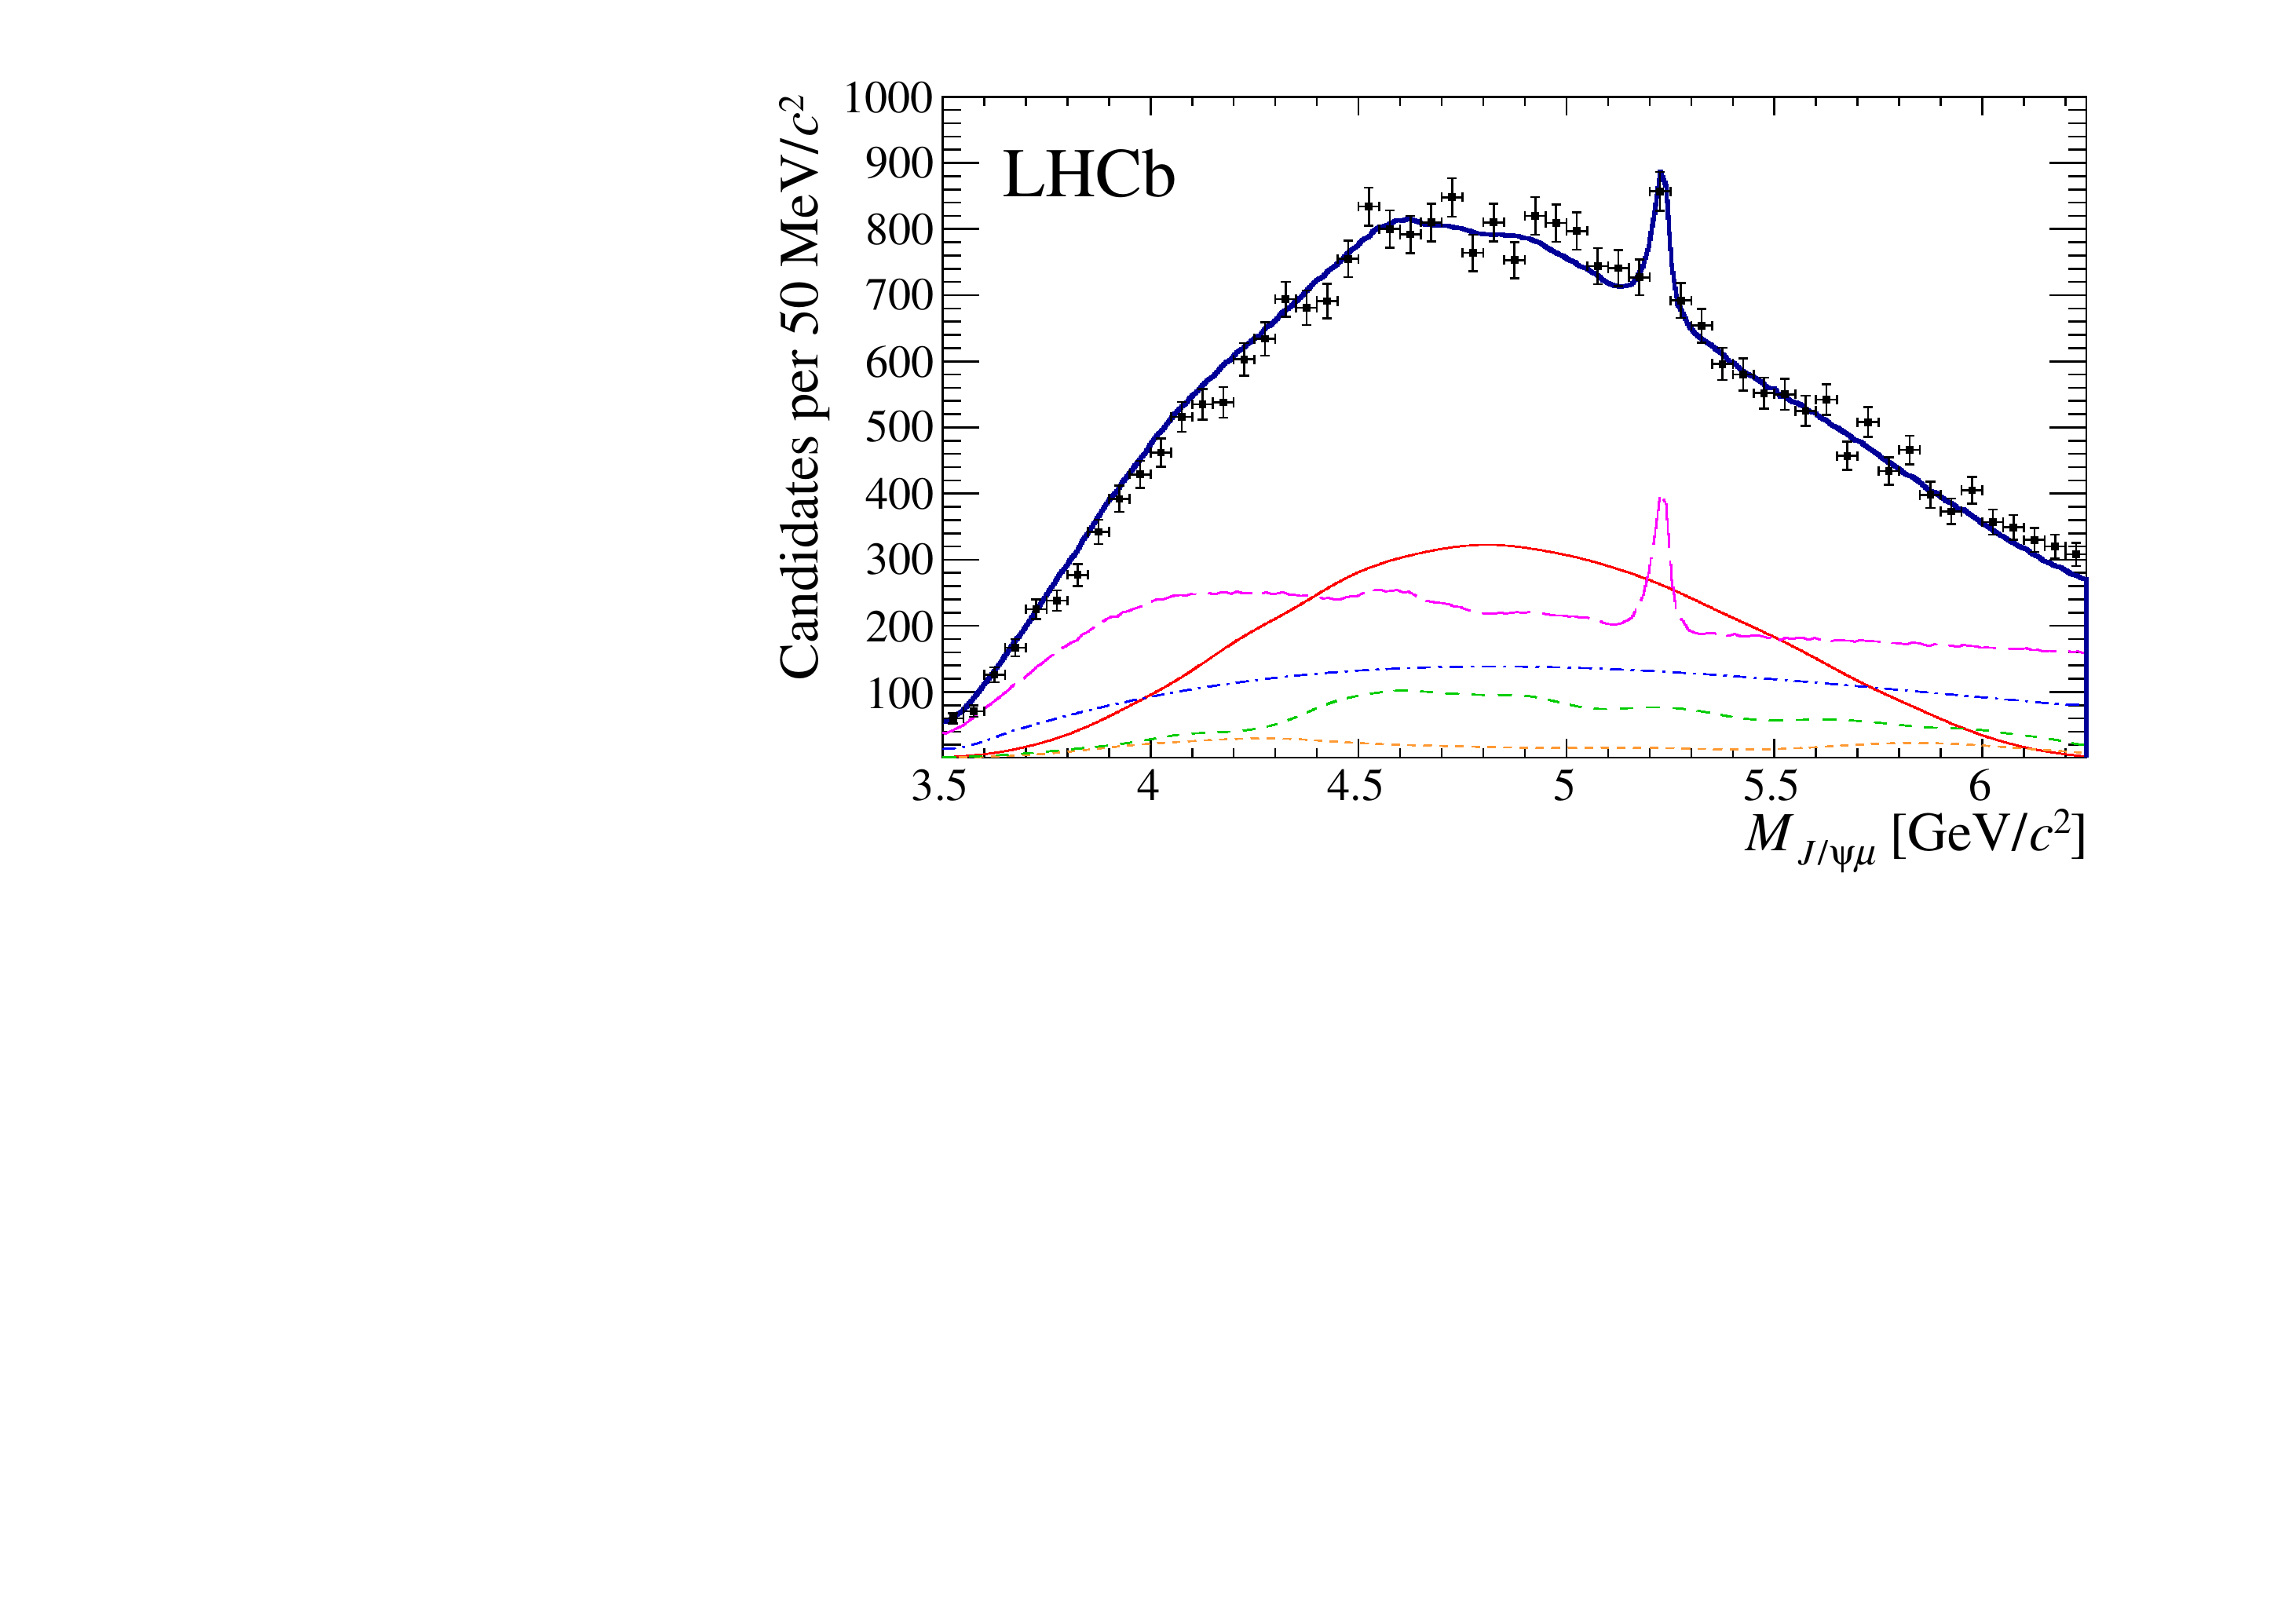}
\put(-60,150){$\mathrm{b})$}\\
\includegraphics[width=.73\textwidth]{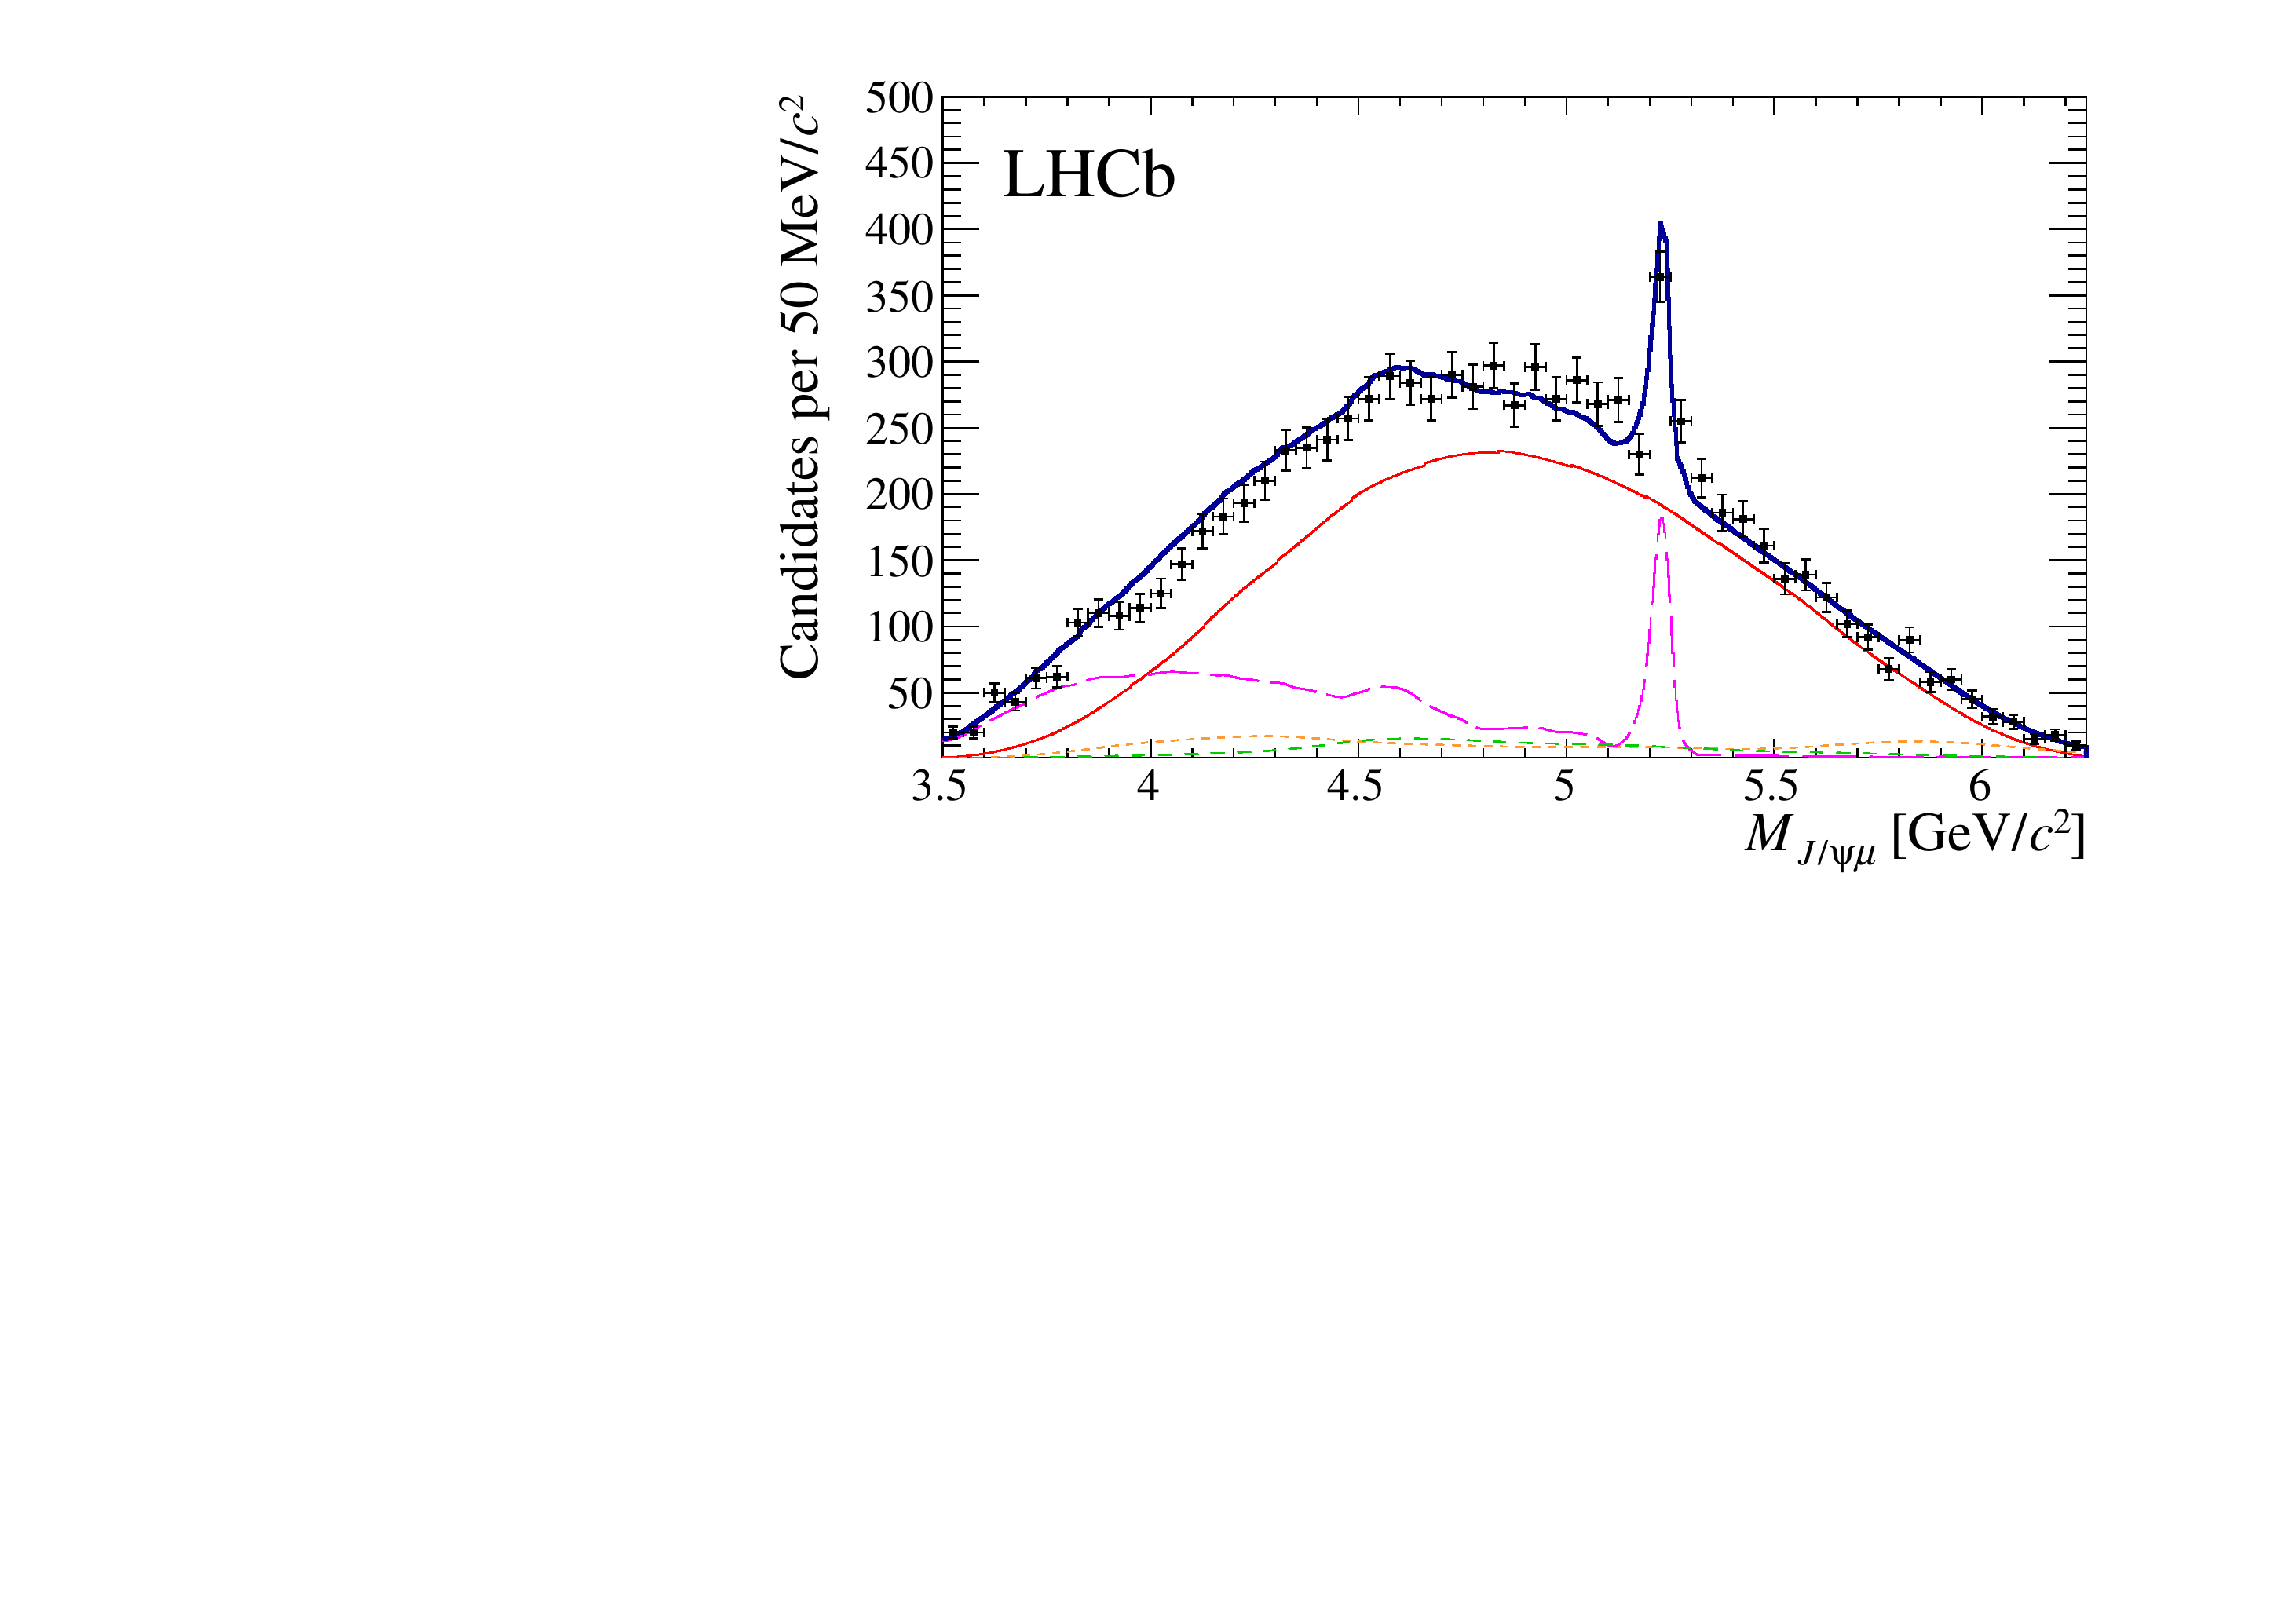}
\put(-60,150){$\mathrm{c})$}\\
  \caption{\small 
    Result of the two-dimensional fit of the \BctojmX model.
    Projections of the total fit function and its components are shown for
    (a) the \pseudot, (b) the mass of all events, and (c) the mass of the detached events ($\pst > 150$~fs).
    This figure is the same as Fig.~\ref{fig:globalfit}, but with a linear scale.
  }
\end{figure}

\begin{figure}[p]
  \centering
\includegraphics[width=.73\textwidth]{img/fig6c_linear.pdf}
\put(-60,150){$\mathrm{a})$}\\
\includegraphics[width=.73\textwidth]{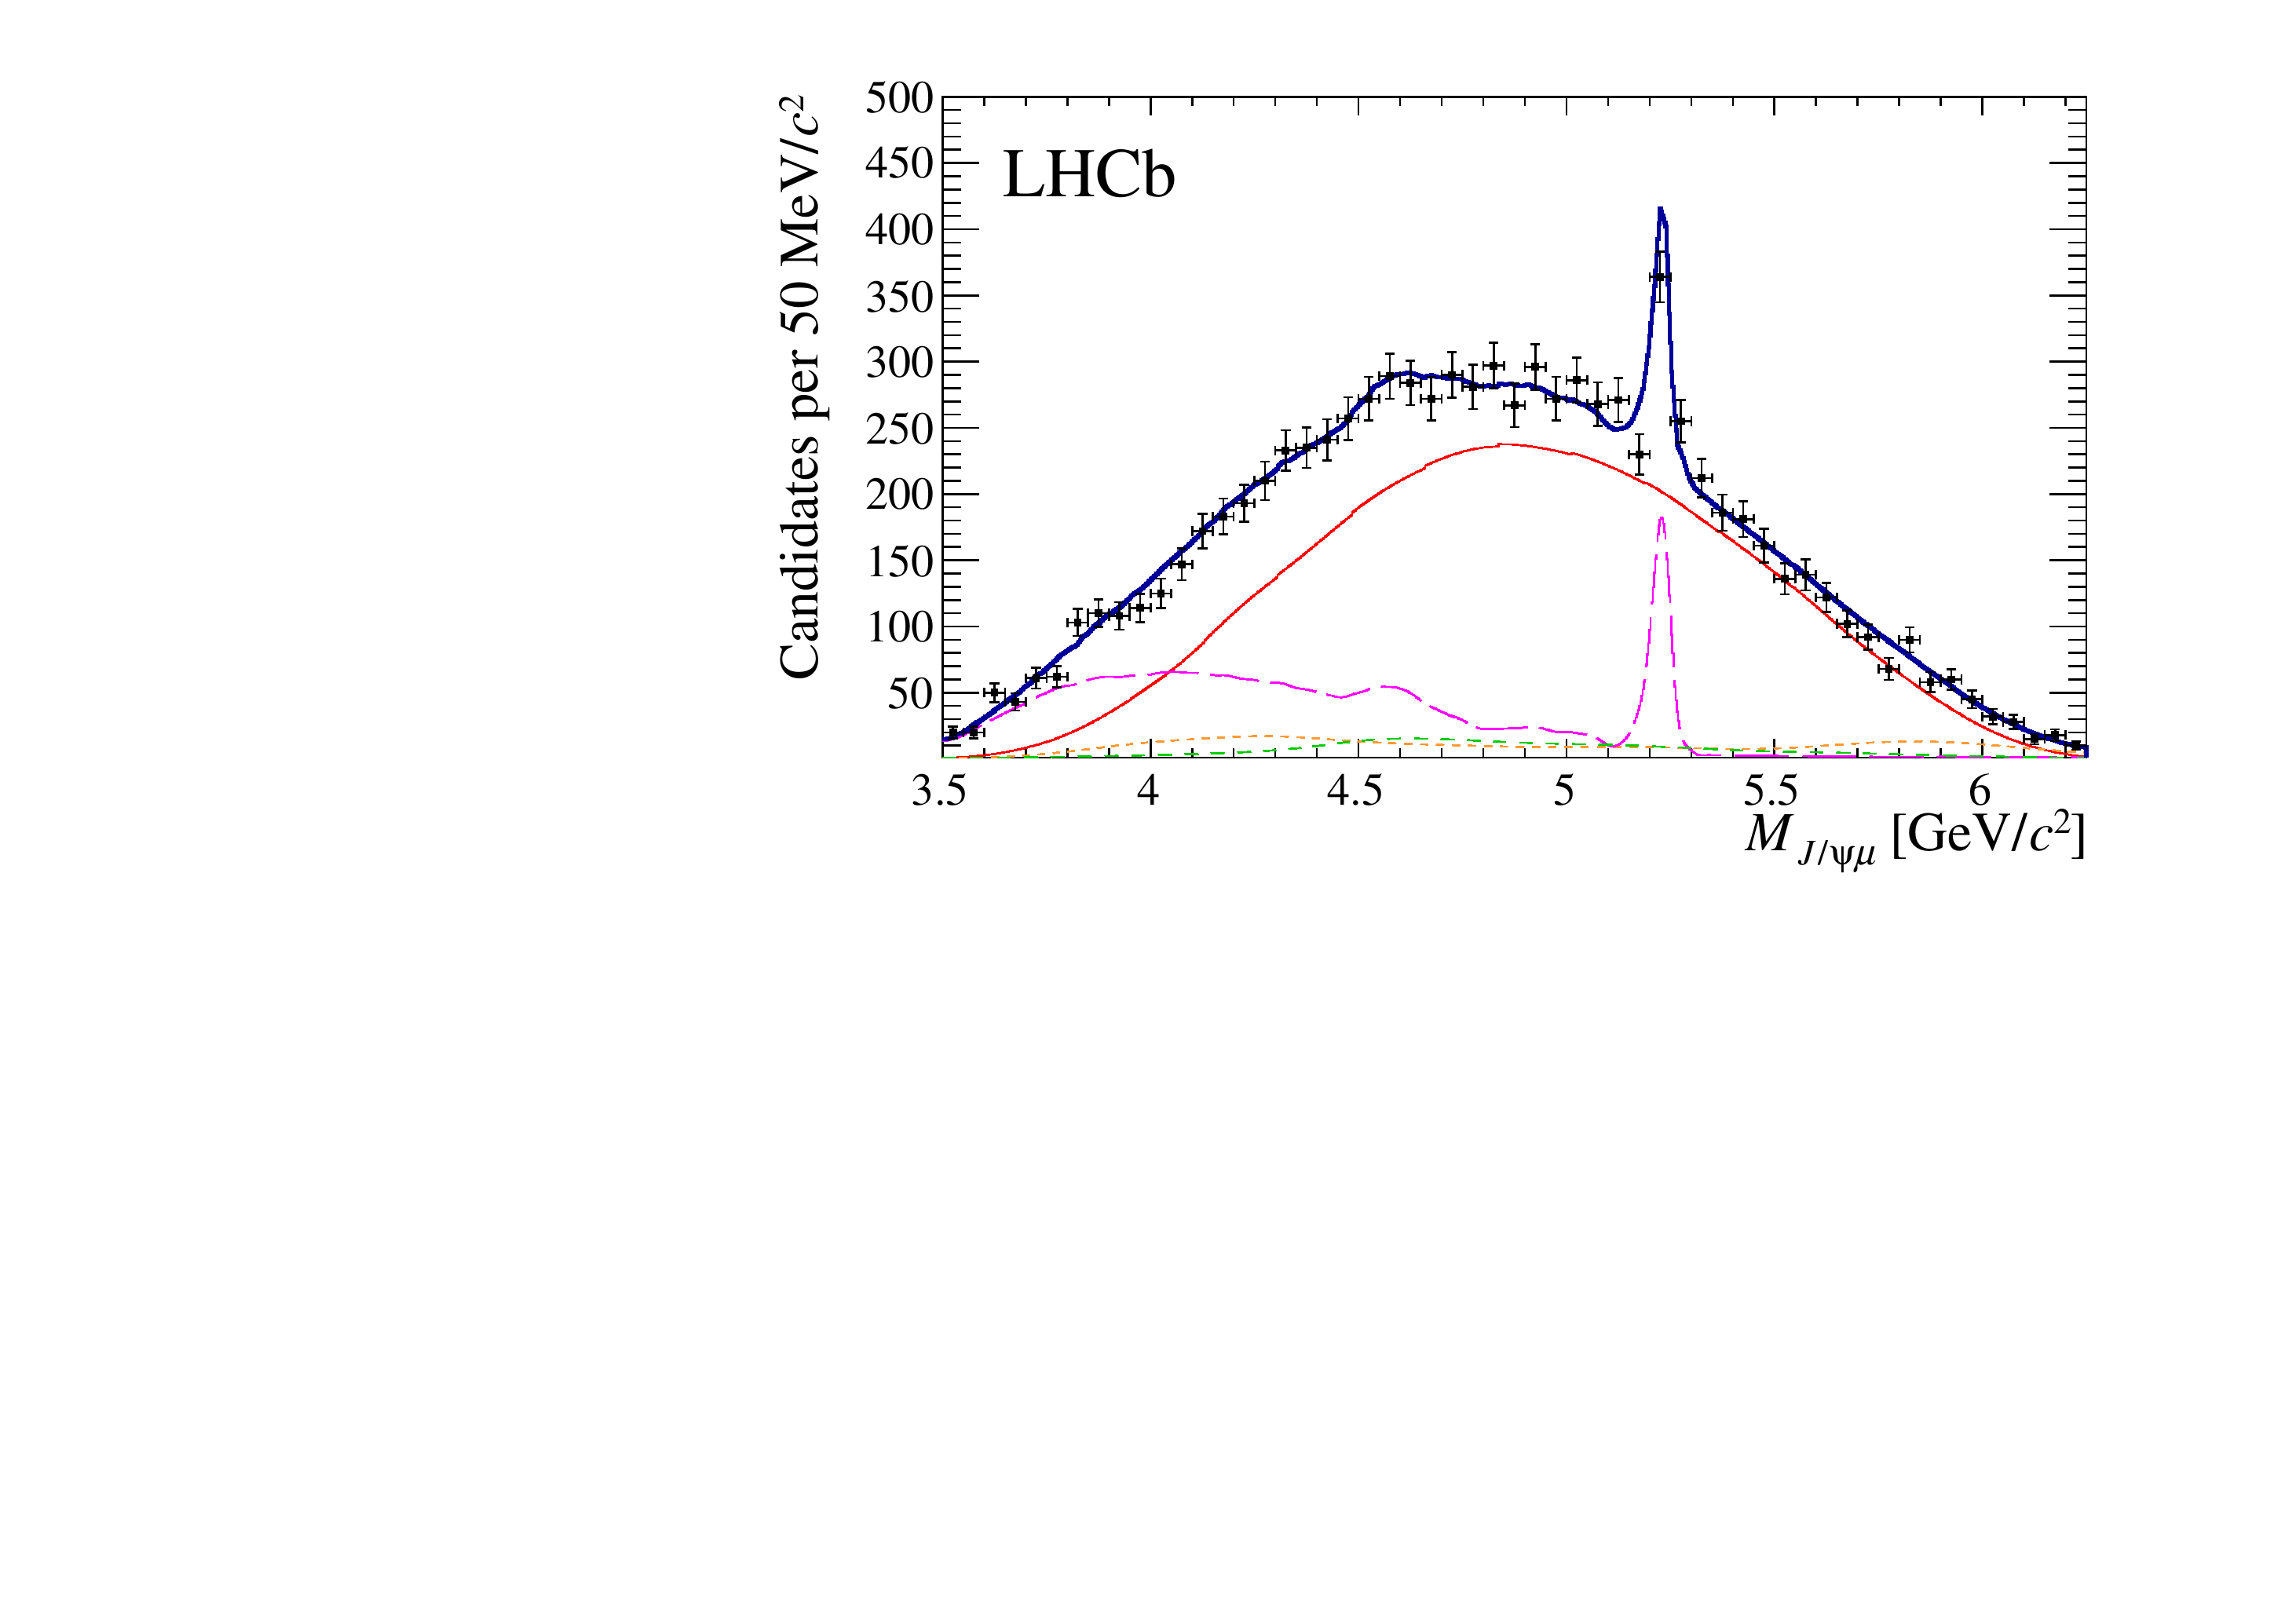}
\put(-60,150){$\mathrm{b})$}\\
  \caption{\small 
    Projections of the total fit function and its components to detached events ($\pst > 150$~fs) 
    in the \Mjm variable (a) for the  nominal fit and (b) after applying
    the deformation of the signal model maximising the agreement with data 
    ($\alpha_\psi = \alpha_\nu$ = 0.3 $c^2\gev^{-1}$ in Eq.~\ref{eq:dalitzdeform}).
    The fit components follow  the legend of Fig.~\ref{fig:globalfit}.
  }
\end{figure}

\clearpage
